# Supplementary material for: A General Framework for Information Extraction using Dynamic Span Graphs
Source: arXiv:1904.03296 source file (2019-04-05)
Supplement: Supplementary file 1 [file Appendix.tex]

% \begin{table}[t]
%   \centering
%  {\small
%   \begin{tabular}{l|llll}
%     \toprule
%      Model & Overlap & Correct & False hit & Miss \\    
%     \midrule
%      SL & 568 & 1064 & 668 & 395\\
%      SSL & 533 & 1193 & 747 & 318\\
%     \bottomrule
%   \end{tabular}}
%   \caption{Error analysis on keyword identification task}
%   \label{tab:span}
% \end{table}
% \newpage
% \newpage
% \clearpage
\begin{appendix}
Paremeter details...
\input{tables/ablation_ace.tex}
\end{appendix}
